# Supplementary material for: SALAD: Part-Level Latent Diffusion for 3D Shape Generation and Manipulation
Source: arXiv:2303.12236 source file (2024-03-20)
Supplement: Supplementary file 1 [file supp_part_completion.tex]

%%%%%%%%%%%%%%%%%%%%%%%%%%%%%%%%
\CatchFileDef{\AllComparisonImages}{figures/part_completion/chair_list.tex}{}
% \graphicspath{{figures/shape_generation/}}

\makeatletter
\def\Image#1{%
  \multicolumn{\LT@cols}{l}{\includegraphics[width=\textwidth]{#1}}\\
}
\makeatother
{
\setlength{\tabcolsep}{0em}

% \newcolumntype{Y}{>{\centering\arraybackslash}X}
\newcolumntype{W}{>{\centering\arraybackslash}m{0.1111\textwidth}}
\newcolumntype{Z}{>{\centering\arraybackslash}m{0.2222\textwidth}}
{\scriptsize
\begin{longtable}{WWW|Z|Z|Z}
GT & Bounding Box & Gaussians & ShapeFormer~\cite{Yan:2022ShapeFormer} & Neural Wavelet~\cite{Hui:2022NeuralWavelet} & \salad{} (Ours) \\ 
  \midrule
  \endhead

  \bottomrule
  \endfoot

  \AllComparisonImages
\end{longtable}
}

\CatchFileDef{\AllComparisonImages}{figures/part_completion/airplane_list.tex}{}
% \graphicspath{{figures/shape_generation/}}

\makeatletter
\def\Image#1{%
  \multicolumn{\LT@cols}{l}{\includegraphics[width=\textwidth]{#1}}\\
}
\makeatother
{
\setlength{\tabcolsep}{0em}

% \newcolumntype{Y}{>{\centering\arraybackslash}X}
\newcolumntype{W}{>{\centering\arraybackslash}m{0.1111\textwidth}}
\newcolumntype{Z}{>{\centering\arraybackslash}m{0.2222\textwidth}}
{\scriptsize
\begin{longtable}{WWW|Z|Z|Z}
GT & Bounding Box & Gaussians & ShapeFormer~\cite{Yan:2022ShapeFormer} & Neural Wavelet~\cite{Hui:2022NeuralWavelet} & \salad{} (Ours) \\ 
  \midrule
  \endhead

  \bottomrule
  \endfoot

  \AllComparisonImages
\end{longtable}
}
%%%%%%%%%%%%%%%%%%%%%%%%%%%%%%%%

%%%%%%%%%%%%%%%%%%%%%%%%%%%%%%%%%%%%%%
% Table class part completion figure %
%%%%%%%%%%%%%%%%%%%%%%%%%%%%%%%%%%%%%%
% \begin{figure*}[h!]
% \centering
% {
% \scriptsize
% \def\arraystretch{0.0}
% \setlength{\tabcolsep}{0em}
% \renewcommand\tabularxcolumn[1]{m{#1}}
% \newcolumntype{W}{>{\centering\arraybackslash}m{0.125\textwidth}}
% \newcolumntype{Z}{>{\centering\arraybackslash}m{0.25\textwidth}}
% \begin{tabularx}{\textwidth}{WWZ|WWZ }
% GT & Gaussians & \salad{} (Ours) & GT & Gaussians & \salad{} (Ours) \\
% \multicolumn{6}{c}{\includegraphics[width=\textwidth]{figures/part_completion/tables/fig-0.png}}\\
% \multicolumn{6}{c}{\includegraphics[width=\textwidth]{figures/part_completion/tables/fig-1.png}}\\
% \multicolumn{6}{c}{\includegraphics[width=\textwidth]{figures/part_completion/tables/fig-2.png}}\\
% \multicolumn{6}{c}{\includegraphics[width=\textwidth]{figures/part_completion/tables/fig-3.png}}\\
% \multicolumn{6}{c}{\includegraphics[width=\textwidth]{figures/part_completion/tables/fig-4.png}}\\
% \multicolumn{6}{c}{\includegraphics[width=\textwidth]{figures/part_completion/tables/fig-5.png}}
% \end{tabularx}
% }
% \end{figure*}
% }
