# Supplementary material for: SALAD: Part-Level Latent Diffusion for 3D Shape Generation and Manipulation
Source: arXiv:2303.12236 source file (2024-03-20)
Supplement: Supplementary file 2 [file iccv_suppl.tex]

\documentclass[10pt,twocolumn,letterpaper]{article}

\usepackage{iccv}
\usepackage{times}
\usepackage{epsfig}
\usepackage{graphicx}
\usepackage{amsmath}
\usepackage{amssymb}
\input{header}
% Include other packages here, before hyperref.

% If you comment hyperref and then uncomment it, you should delete
% egpaper.aux before re-running latex.  (Or just hit 'q' on the first latex
% run, let it finish, and you should be clear).
\usepackage[breaklinks=true,bookmarks=false]{hyperref}

\iccvfinalcopy % *** Uncomment this line for the final submission

 % *** Enter the ICCV Paper ID here

% Pages are numbered in submission mode, and unnumbered in camera-ready
\ificcvfinal\pagestyle{empty}\fi

\begin{document}
\onecolumn
%%%%%%%%% TITLE
\title{SALAD: Part-Level Latent Diffusion for 3D Shape Generation and Manipulation --- Supplementary Material}

\author{Juil Koo\textsuperscript{$\ast$} $\quad$
Seungwoo Yoo\textsuperscript{$\ast$} $\quad$
% Minh Hieu Nguyen\textsuperscript{*} $\quad$
Minh Hieu Nguyen\textsuperscript{$\ast$} $\quad$
Minhyuk Sung \\
KAIST\\
{\tt\small \{63days,dreamy1534,hieuristics,mhsung\}@kaist.ac.kr}
}

\maketitle
% Remove page # from the first page of camera-ready.
\ificcvfinal\thispagestyle{empty}\fi

\def\thefootnote{*}\footnotetext{Equal contribution.}\def\thefootnote{\arabic{footnote}}

\renewcommand{\thesection}{S}
\renewcommand{\thetable}{S\arabic{table}}
\renewcommand{\thefigure}{S\arabic{figure}}

\newif\ifpaper
\input{iccv2023AuthorKit/sections/999_Supplementary}

{\small
\bibliographystyle{ieee_fullname}
\bibliography{egbib}
}

\end{document}
